# Supplementary material for: Extend Your Own Correspondences: Unsupervised Distant Point Cloud Registration by Progressive Distance Extension
Source: arXiv:2403.03532 source file (2024-03-27)
Supplement: Supplementary file 1 [file X_supp_original.tex]

\clearpage
\setcounter{page}{1}
\maketitlesupplementary

% \textcolor{red}{Note: This supplementary is not complete in its current version.}

\section{Additional Experiments}
\subsection{Detailed Experiment Setup}
\paragraph{Comparison methods.} Considering the lack of genuine unsupervised distant point cloud registration methods at present, we compare EYOC against supervised methods instead. The most compared baselines are the two fully-convolutional methods, FCGF \cite{choy2019fully} and Predator \cite{huang2021predator}. The former utilizes MinkowskiNet for sparse voxel convolution, while the latter builds upon KPConv which classifies as a point convolution method. On the other hand, performances of SpinNet \cite{ao2021spinnet}, D3Feat \cite{bai2020d3feat}, CoFiNet \cite{yu2021cofinet}, and GeoTransformer \cite{qin2022geometric} are quoted verbatim from GCL \cite{liu2023density}.

\paragraph{Formal definition for metrics.} Given a test set with labels $X_{[d_1,d_2]}=\left\{(S^i,T^i, R^i, t^i)\big|\ ||t^i||_2\in [d_1,d_2]\right\}$ where $S^i,T^i$ are point clouds and $R^i\in SO(3),t^i\in \mathbb{R}^3$ are the ground truth transformation, along with the estimated transformation $\hat{R}^i, \hat{t}^i$, the absolute rotational error and absolute translational error are defined as \cref{eq:re,eq:te}. Please note that we abbreviate $X$ for ${X_{[d_1,d_2]}}$ hereafter to save space where the subscript does not matter.

\begin{equation}
    \mathbf{RE}^{i}_{X} = \arccos{\left(\frac{trace({R^i}^T\hat{R}^i)-1}{2}\right)} \\
    \label{eq:re}
\end{equation}

\begin{equation}
    \mathbf{TE}^{i}_{X} = ||t^i - \hat{t}^i|| \\
    \label{eq:te}
\end{equation}

It is generally observed that, when registration performs well, these errors are usually limited and predictable; However, they could drift randomly during failures, often leading to more than $90\degree$ or $50m$ of error. It is neither interpretable nor repeatable to average the error over all the pairs containing occasional arbitrarily large errors; On the contrary, we often choose to average only those errors of the successful pairs. The registration success is assessed based on the criterion of $S(X,i)=\mathds{1}(RE^{i}_{X}<T_{rot})\times\mathds{1}(TE^{i}_X<T_{trans})$, where $\mathds{1}(\cdot)$ is the Iverson Bracket, and $T_{rot}=5\degree, T_{trans}=2m$ are two generally accepted thresholds. After that, we could calculate the RRE, RTE as the average of RE and TE of succeeded pairs, and RR as the portion of successful pairs over all pairs, as formulated in \cref{eq:rre,eq:rte,eq:rr}:

\begin{equation}
    \mathbf{RRE}_{X} = \frac{1}{\sum\limits_{i=1}^{|X|} S(X,i)}\sum\limits_{i=1}^{|X|} \left(S(X,i) \times \mathbf{RE}^{i}_{X}\right)\\
    \label{eq:rre}
\end{equation}

\begin{equation}
    \mathbf{RTE}_{X} = \frac{1}{\sum\limits_{i=1}^{|X|} S(X,i)}\sum\limits_{i=1}^{|X|} \left(S(X,i) \times \mathbf{TE}^{i}_{X}\right)\\
    \label{eq:rte}
\end{equation}

\begin{equation}
    \mathbf{RR}_{X} = \frac{1}{|X|}\sum\limits_{i=1}^{|X|} S(X,i)\\
    \label{eq:rr}
\end{equation}

Next, mRR is defined as the average of RR over five registration subsets with $||t||\in [d_1,d_2]$ meters,  and the tuple $(d_1,d_2)$ is parameterized according to our specification, \textit{i.e.}, $D_{V2V}=\{(5,10), (10,20), (20,30), (30,40), (40,50)\}$, respectively according to \cref{eq:mrr}:

\begin{equation}
    \mathbf{mRR} = \frac{1}{|D_{V2V}|}\sum\limits_{(d_1,d_2)\in D_{V2V}} \mathbf{RR}_{X_{[d_1,d_2]}}\\
    \label{eq:mrr}
\end{equation}

Lastly, given a dataset $X$ and the estimated correspondences $(j,k)\in C^i$ denoting that $p^j\in S^i, q^k\in T^i$ are a pair of correspondence, the inlier ratio is defined as \cref{eq:ir}:

\begin{equation}
    \mathbf{IR}_{X} = \sum\limits_{i=1}^{|X|} \sum\limits_{(j,k)\in C^i}\frac{\mathds{1}(||R^ip^j+t^i-q^k|| \leq T_{inlier})}{|X|\times |C^i|}\\
    \label{eq:ir}
\end{equation}

Where $T_{inlier}=0.3m$ is the inlier distance threshold.

% \subsection{Continuous Dataset Setup}
% \label{sec:appendix_continuous_dataset}
\subsection{Performance on Other Benchmarks}

\begin{table}[t]
    \centering
    \small
    \resizebox{\linewidth}{!}{
      \begin{tabular}{@{}lccc|ccc@{}}
        \toprule
        \multirow{2}{*}{Method} & \multicolumn{3}{c|}{KITTI$[10,10]$} & \multicolumn{3}{c}{LoKITTI}\\
        \cmidrule{2-7}
        & RR & RRE & RTE & RR & RRE & RTE\\
        %   & Loading &Extracton & Generation & Prop. & Passes\\
        \midrule
FCGF \cite{choy2019fully}	        &97.8	&0.35	&12.6    &22.2	&2.02	&55.2\\
FCGF+APR \cite{ijcai2023p134}	    &98.2	&0.34	&9.6     &32.7	&1.74	&51.9\\
Predator \cite{huang2021predator}	&100.0	&0.31	&7.4     &42.4	&1.75	&43.4\\
Predator+APR \cite{ijcai2023p134}	&100.0	&0.30	&7.3     &50.8	&1.64	&39.5\\
GCL+Conv \cite{liu2023density}	    &98.6	&0.26	&6.6     &72.3	&1.03	&25.9\\
GCL+KPConv \cite{liu2023density}	&99.2	&0.25	&7.5     &55.4	&1.28	&27.8\\
EYOC (ours)                         &98.5   &0.27   &7.8     &42.2  & 1.48  & 29.2\\
        
        \midrule
        \midrule

        & \multicolumn{3}{c|}{nuScenes$[10,10]$} & \multicolumn{3}{c}{LoNuScenes}\\
        %   & Loading &Extracton & Generation & Prop. & Passes\\
        \midrule
FCGF \cite{choy2019fully}	        &93.6	&0.46	&50.0    &49.1	&1.30	&60.9\\
FCGF+APR \cite{ijcai2023p134}	    &94.5	&0.45	&37.0    &51.8	&1.40	&62.0\\
Predator \cite{huang2021predator}   &97.8	&0.58	&20.2    &50.4	&1.47	&54.5\\
Predator+APR \cite{ijcai2023p134}   &99.5	&0.47	&19.1    &62.7	&1.30	&51.8\\
GCL+Conv \cite{liu2023density}	    &99.2	&0.30	&16.7    &82.4	&0.70	&46.8\\
GCL+KPConv \cite{liu2023density}	&99.7	&0.35	&15.9    &86.5	&0.84	&46.5\\
EYOC (ours)                         &97.8   &0.36   &19.9    &53.2  &0.96   &48.8 \\
        \bottomrule
      \end{tabular}
     }
    \caption{Performance of SOTA distant point cloud registration methods and EYOC. Baselines are quoted verbatim from \cite{liu2023density}.}
    \label{tab:low_overlap_tests}
\end{table}

We display the performance of EYOC among other distant point cloud registration methods on four common baselines, including high-overlap benchmarks KITTI[10,10], nuScenes[10,10] \cite{choy2019fully, huang2021predator} and low-overlap benchmarks LoKITTI, LoNuScenes \cite{ijcai2023p134} in \cref{tab:low_overlap_tests}. Judging from the low-overlap datasets, we see that EYOC achieves comparable performance with the methods other than GCL who densely utilized the label information, achieving $42.2\%$ ($-0.2\%$) and $53.2\%$ ($+2.8\%$) RR on LoKITTI and LoNuScenes compared to the best non-dedicated method Predator, while slightly lagging behind other superior supervised methods in the long-range scenarios. On the other hand, all methods performed similarly well in the high-overlap scenarios, often surpassing $98\%$ RR. We conclude that while EYOC lags behind SOTA supervised distant point cloud registration methods, our method still achieves comparable performance with its comparable baselines.

\subsection{Effect of Extension Step Size}
We display the performance of EYOC when $B$ in the progressive dataset grows in larger steps, ranging from 2 to 15 frames, compared with the default setup where $B$ always grows by one, as listed in \cref{tab:extension_step_size}. While the default interval of 1 frame performs the best at $68.8\%$ RR, other setups with larger steps perform consistently worse at $65.3\%$ RR where the steps lie between $2$ and $5$ frames, and larger steps further impair network performance when $B=8$ or $B=15$. We conclude that an utmost smooth distance extension step grants the best scores, which entitles our default setting.

\begin{table}[t]
    \centering
    \small
    \resizebox{\linewidth}{!}{
      \begin{tabular}{@{}lccccccc@{}}
        \toprule
        Step Size (Frames) & 1 & 2 & 3 & 4 & 5 & 8 & 15\\
        %   & Loading &Extracton & Generation & Prop. & Passes\\
        \midrule
        RR @$d\in [40,50]$ & 68.8 & 65.3 & 65.3 & 65.3 & 65.3 & 64.8 & 56.8\\
        \bottomrule
      \end{tabular}
     }
    \caption{Effect of the extension step size for EYOC on KITTI. Larger steps contribute negatively to network performance.}
    \label{tab:extension_step_size}
\end{table}

\subsection{Rationale for the Progressive Distance Extension Strategy}
In all three datasets \cite{Geiger2012CVPR,Caesar_2020_CVPR,Sun_2020_CVPR}, the curves of maximum point cloud distance relative to frame interval are roughly linear as depicted in \cref{fig:frame_dist_plot}. As our investigations reveal, all datasets have their maximum translation over 50m after the interval reaches 30 frames. We conclude that setting the frame interval bound $B$ to 30 frames would be a decent choice to guarantee coverage of the long-range pairs on most of the mainstream LiDAR point cloud datasets.

\begin{figure}[t]
  \centering
  \includegraphics[width=0.9\linewidth]{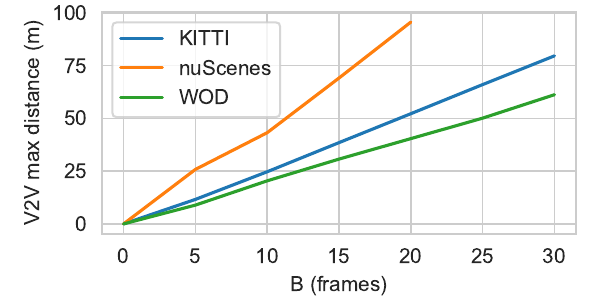}
  \vspace{-0.3cm}
  \caption{\textbf{The relation between maximum point cloud distance and the maximum frame interval $B$.} 30 Frames are enough to cover all scenarios of distant point cloud registration (\textit{i.e.}, up to 50m apart).}
  \label{fig:frame_dist_plot}
%   \vspace{-0.4cm}
\end{figure}

\section{Discussions}

\subsection{More on Hypothesis \ref{hyp:corr}}
\label{sec:appendix_proofs}
\paragraph{Non-linear cases.} Expanding the definitions of \cref{sec:hypothesis}, where the point $p=(a,b,0)^T$ is observed from the current LiDAR center $O=(0,0,0)^T$, we now move the LiDAR in all three directions to $O'=(x,y,z)^T$. We calculate the density change as $\Delta\sigma_p=\frac{\alpha}{(a-x)^2+(b-y)^2+z^2}-\frac{\alpha}{a^2+b^2}$. We do notice that now closer-to-LiDAR points do not necessarily experience a bigger fluctuation in density; It now rather depends on the direction of translation. We explain this phenomenon by visualizing the absolute density change $\left|\Delta \sigma_p\right|$ on a $100m\times 100m$ canvas when the LiDAR center moves from $O=(0,0,0)^T$ to $O'=(10,10,5)^T$, as illustrated in \cref{fig:translation_density}. Near the mid vertical of the line segment $OO'$, the density changes are close to none due to having approximately the same distance to $O$ and $O'$. However, we still observe aggressive density changes near the LiDAR positions, $O=(0,0,0)^T$ and $O'=(10,10,5)^T$, which confirms that our hypothesis holds true. Additionally, the peak around $O'$ is lower due to a vertical distance of 5 meters above the $a-b$ plane.

\begin{figure}[t]
  \centering
  \vspace{0.3cm}
  \begin{overpic}[scale=0.7]{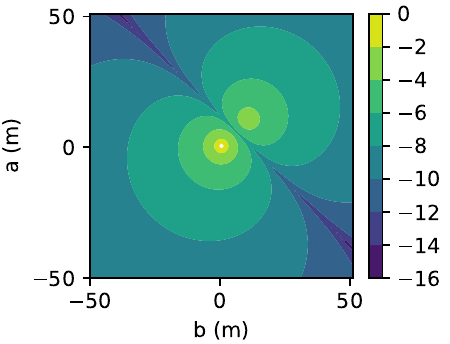}
  \put(80,77){\footnotesize $\alpha\times 10^{(\cdot)}$}
  \end{overpic}
  \vspace{-0.3cm}
  \caption{The density change $\Delta\sigma_p$ for any point on the horizontal plane when the LiDAR center moves from origin to $(10,10,5)^T$. Values are shown with brightness in log scale. Far-away regions suffer less density variation overall.}
  \label{fig:translation_density}
%   \vspace{-0.4cm}
\end{figure}

\paragraph{Discussions on our assumption.} We further discuss our assumption that the vehicle translation distance should be quite limited compared to the observed point distance $||p||$.
Presumably, as we arrange the progressive dataset to grow by tiny steps, \textit{i.e.}, $B$ grows by one every 6.7 epochs and accumulates to 30 in 200 epochs, we would expect the network to face a limited growth in point cloud distance. According to \cref{fig:frame_dist_plot}, even in nuScenes with the most rapid movements, one frame interval would correspond to at most 5 meters of driving distance. Granted that LiDARs generally have over 80 meters of scope on the $x-y$ plane and have the near regions cut off around the LiDAR due to temporal resolution constraints, we should conclude that our assumption largely holds.

\paragraph{Compatibility with previous literature.} Moreover, we notice that Hypothesis \ref{hyp:corr} would hint that point cloud features would deteriorate (\textit{i.e.}, move) on the feature space slower than linear functions relative to the distance-to-LiDAR (\textit{e.g.}, radical functions). We argue that this does not contradict previous literature \cite{liu2023density} which found the relation to be linear; While previous literature looked into the in-domain performance of converged models, we are looking into the out-of-domain performance of models during training. It is natural for networks to behave differently on seen and unseen data.

\begin{figure}[t]
  \centering
%   \vspace{-0.2cm}
%   \includegraphics[width=\linewidth]{figure/analysis.pdf}
  \includegraphics[width=\linewidth]{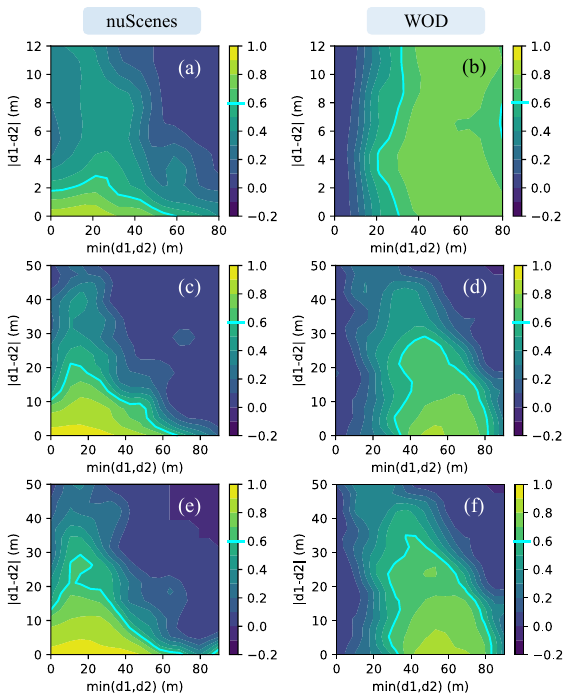}
  \vspace{-0.7cm}
  \caption{\textbf{Visual groundings} for our hypothesis on (a,c,e) nuScenes \cite{Caesar_2020_CVPR} and (b,d,f) WOD \cite{Sun_2020_CVPR}. Cosine similarity of correspondences with its distance to two LiDARs, $d_1, d_2$, is displayed for $I\in [1,1]$ (top), $I\in [1,15]$ (middle), and $I\in [1,30]$ (bottom). Decision boundaries at $s_{thresh}=0.6$ are highlighted in cyan.}
  \label{fig:dist_sim_nus_wod}
  \vspace{-0.2cm}
\end{figure}

% \subsection{More on Time Analysis}
% \label{sec:appendix_time_analysis}
% We further explain why EYOC has a lower training time than its supervised counterpart, FCGF \cite{choy2019fully}. As pointed out in \cref{sec:time}, threaded dataloaders are not allowed to use GPU as specified in Pytorch, but we do notice that canceling the threading enables GPUs in dataloaders, meaning that we actually can perform NN-search on GPU for FCGF. However, this cancels the boost caused by pipelining multiple dataloader threads with the trainer thread, resulting in a surge of data loading time to $1885$ms instead. The only reasonable choice is to make drastic changes to the original code, moving the NN-search step to the trainer thread completely with the help of Pytorch3D, which would result in a time consumption similar to that of EYOC.

\section{Visualization}

\subsection{Spatial Filtering on other Datasets}
\label{sec:appendix_other_datasets}
We display the spatial feature similarity results on WOD and nuScenes in \cref{fig:dist_sim_nus_wod}, where $d_1, d_2$ denotes the distance from a correspondence to the two LiDAR centers, and the similarity is indicated by brightness. The decision boundary of $s_thresh=0.6$ is highlighted in cyan, similar to \cref{fig:theoretical_similarity}. WOD exhibits almost identical traits to those on KITTI, showing a drastic feature deterioration in the close-to-LiDAR regions as well as the extremely far regions, and cutting off at 40m would almost always cut the closer half below 0.6 similarity, indicating the similarity between the two filtering strategies. On the other hand, nuScenes displays a similar pattern where high-similarity regions are clustered 20 meters away from the LiDAR. Compared to those on KITTI or WOD, the pinnacle region in nuScenes is slightly shifted towards the LiDAR compared with the other two datasets, due to the lower LiDAR resolution and consequently lower density. In nuScenes, it would be improper to cut off at 40m, although the training does converge and has decent performance as reported in \cref{tab:comparison}. While this phenomenon is attributed to the discrepancy between KITTI-style datasets and nuScenes-style datasets, we also highlight that EYOC is robust under such discrepancies even when the patterns for the pretraining dataset (WOD) largely differ from the actual one on the finetuning dataset (nuScenes).

\subsection{Registration Results}
We display the registration results of EYOC on KITTI, nuScenes and WOD in \cref{fig:reg_results_kitti,fig:reg_results_nuscenes,fig:reg_results_waymo}.

\begin{figure*}[t]
  \centering
  \includegraphics[width=0.45\linewidth]{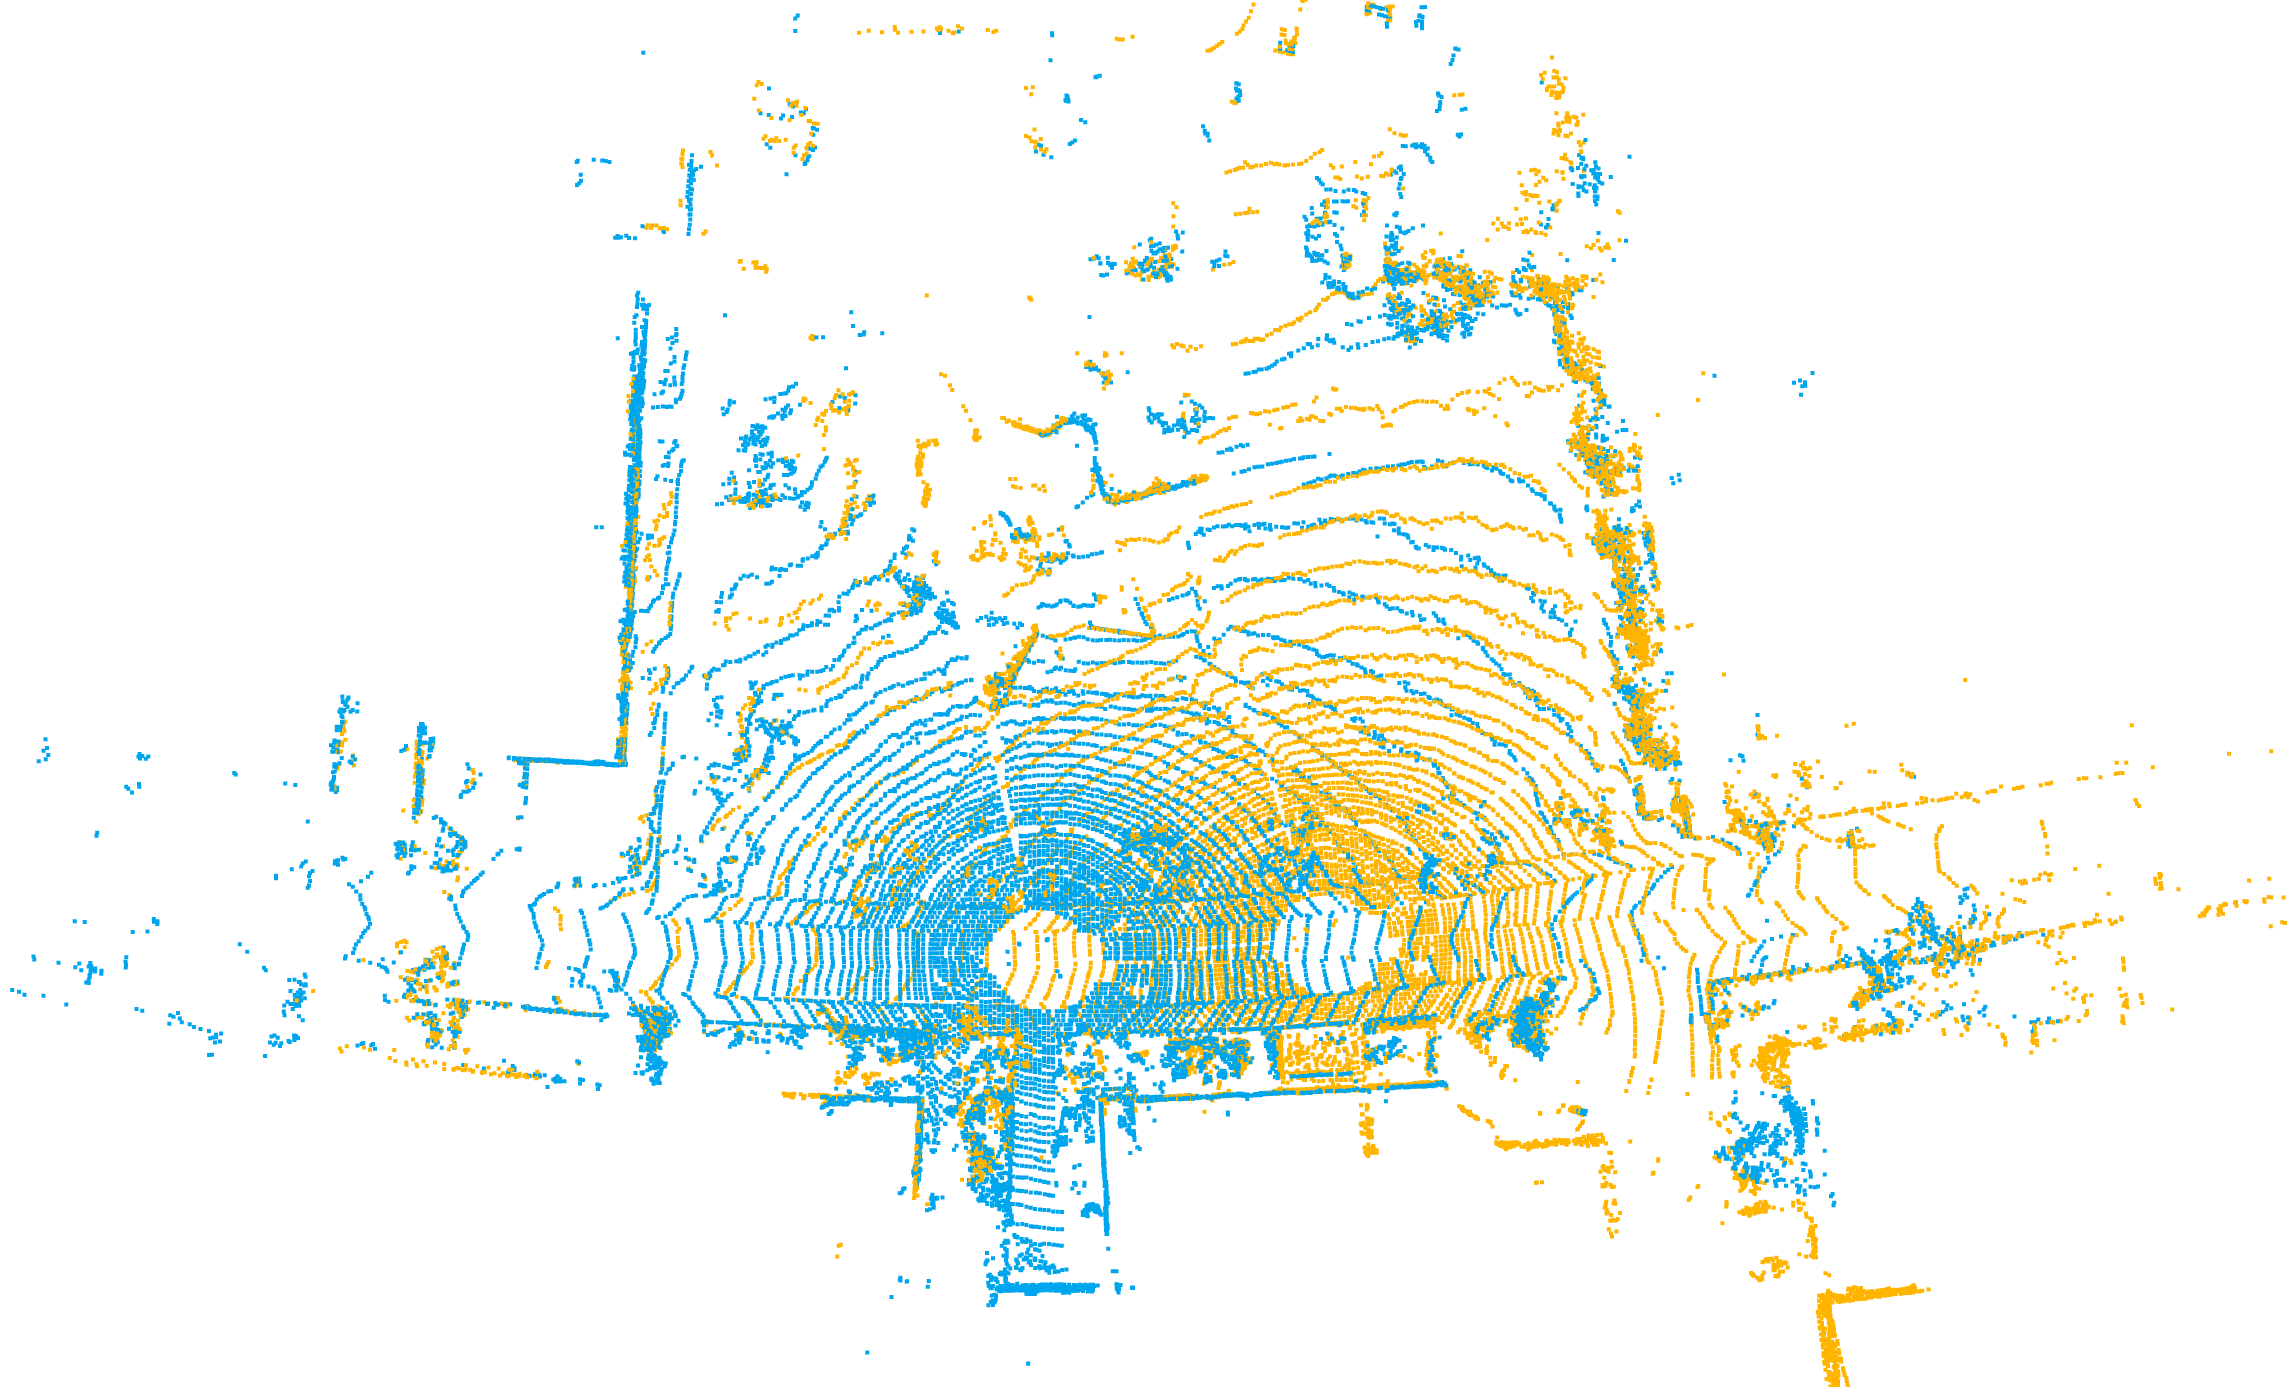} \hfill
  \includegraphics[width=0.45\linewidth]{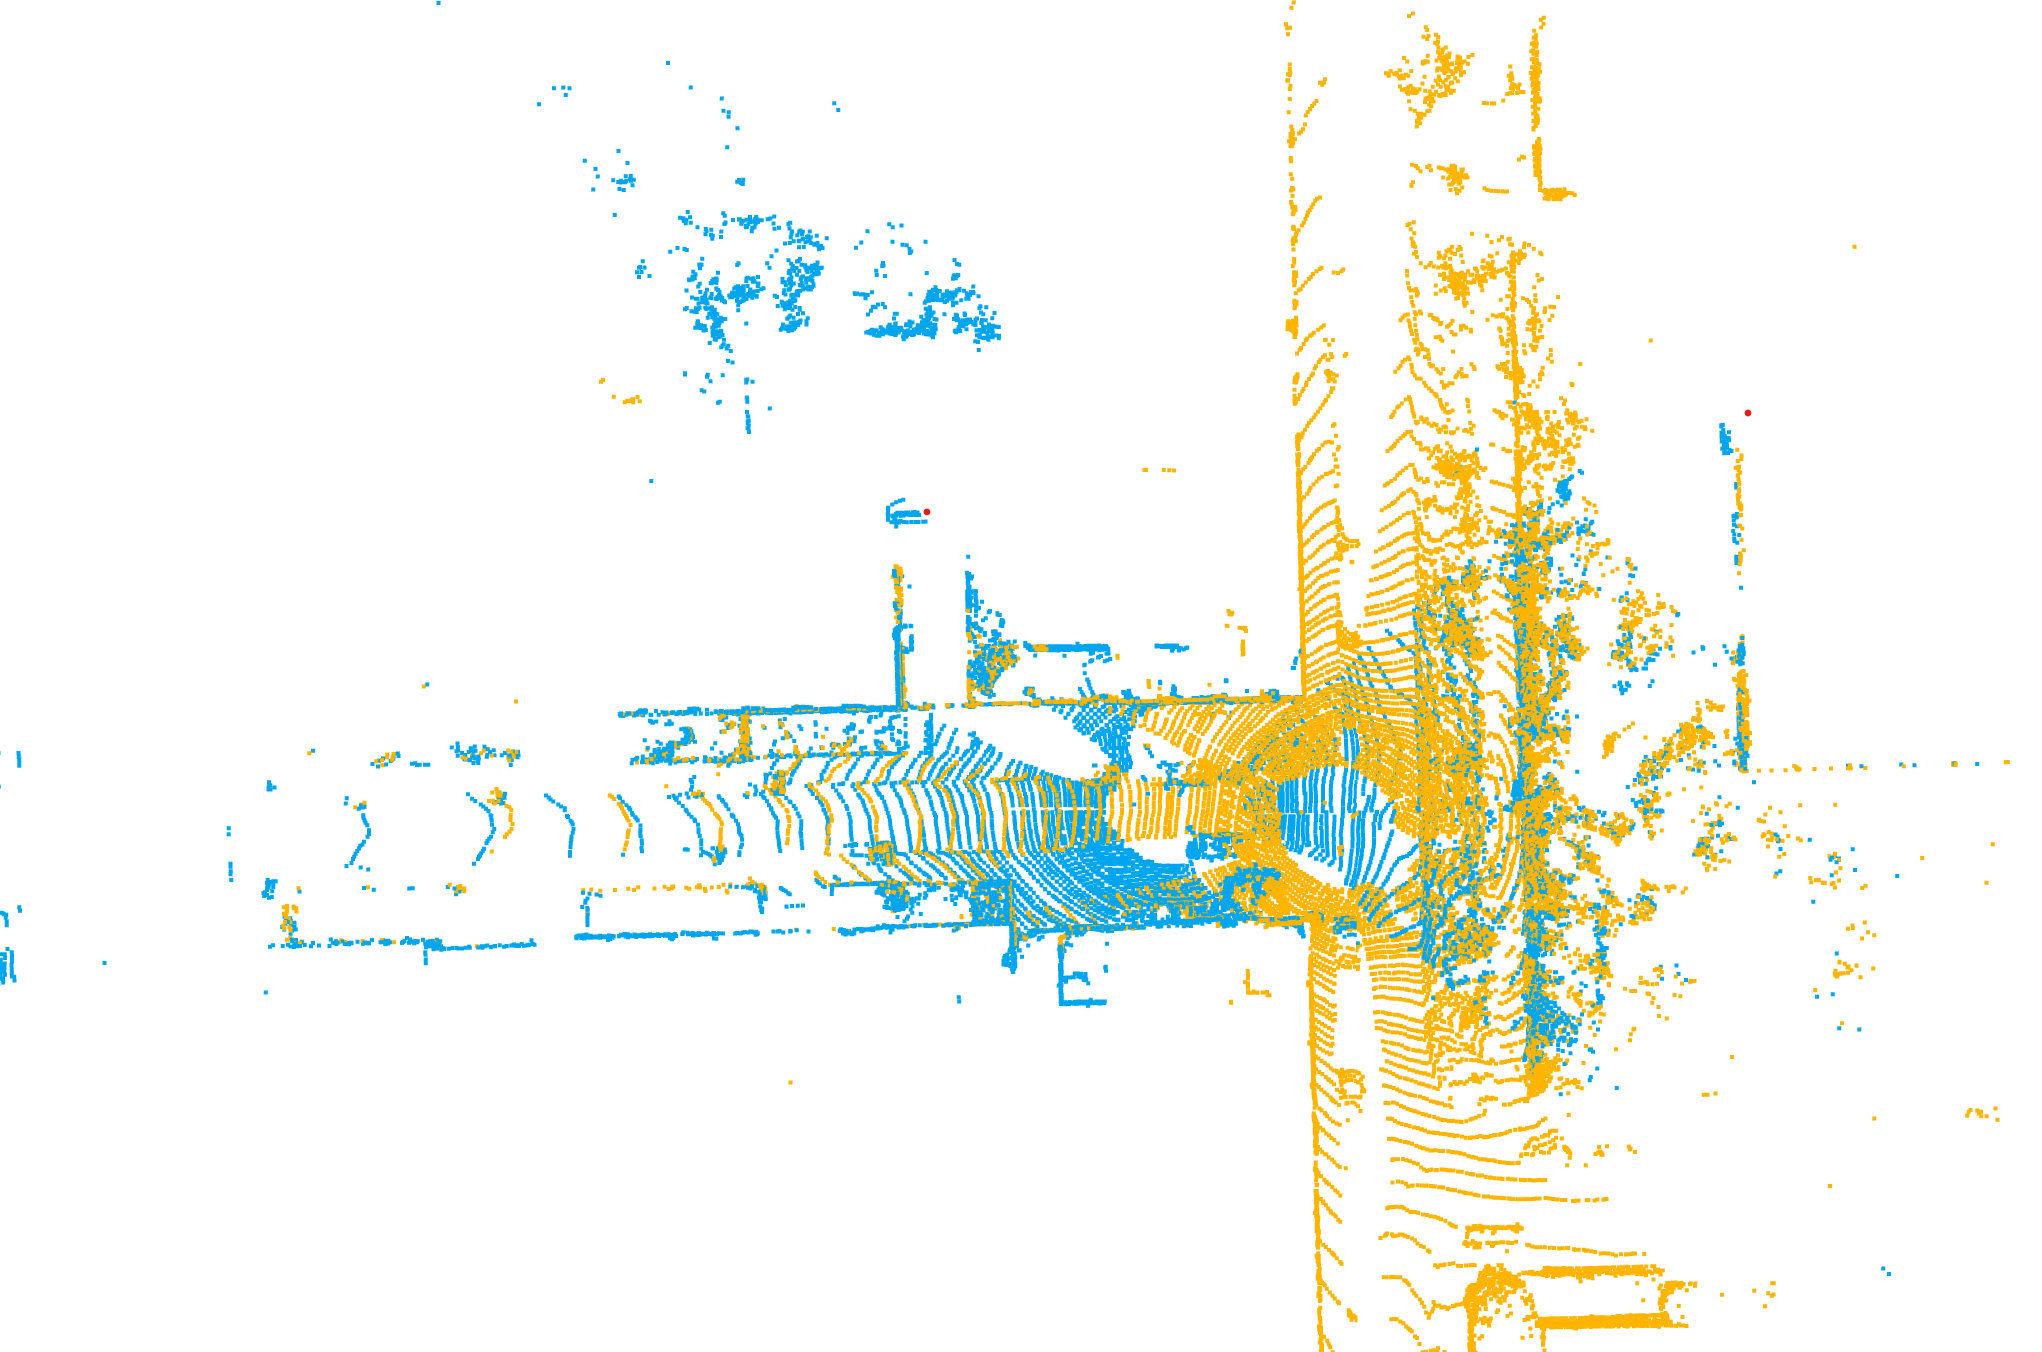} \hfill
  \caption{Registration results of EYOC on KITTI \cite{Geiger2012CVPR}.}
  \label{fig:reg_results_kitti}
%   \vspace{-0.2cm}
\end{figure*}

\begin{figure*}[t]
  \centering
  \includegraphics[width=0.45\linewidth]{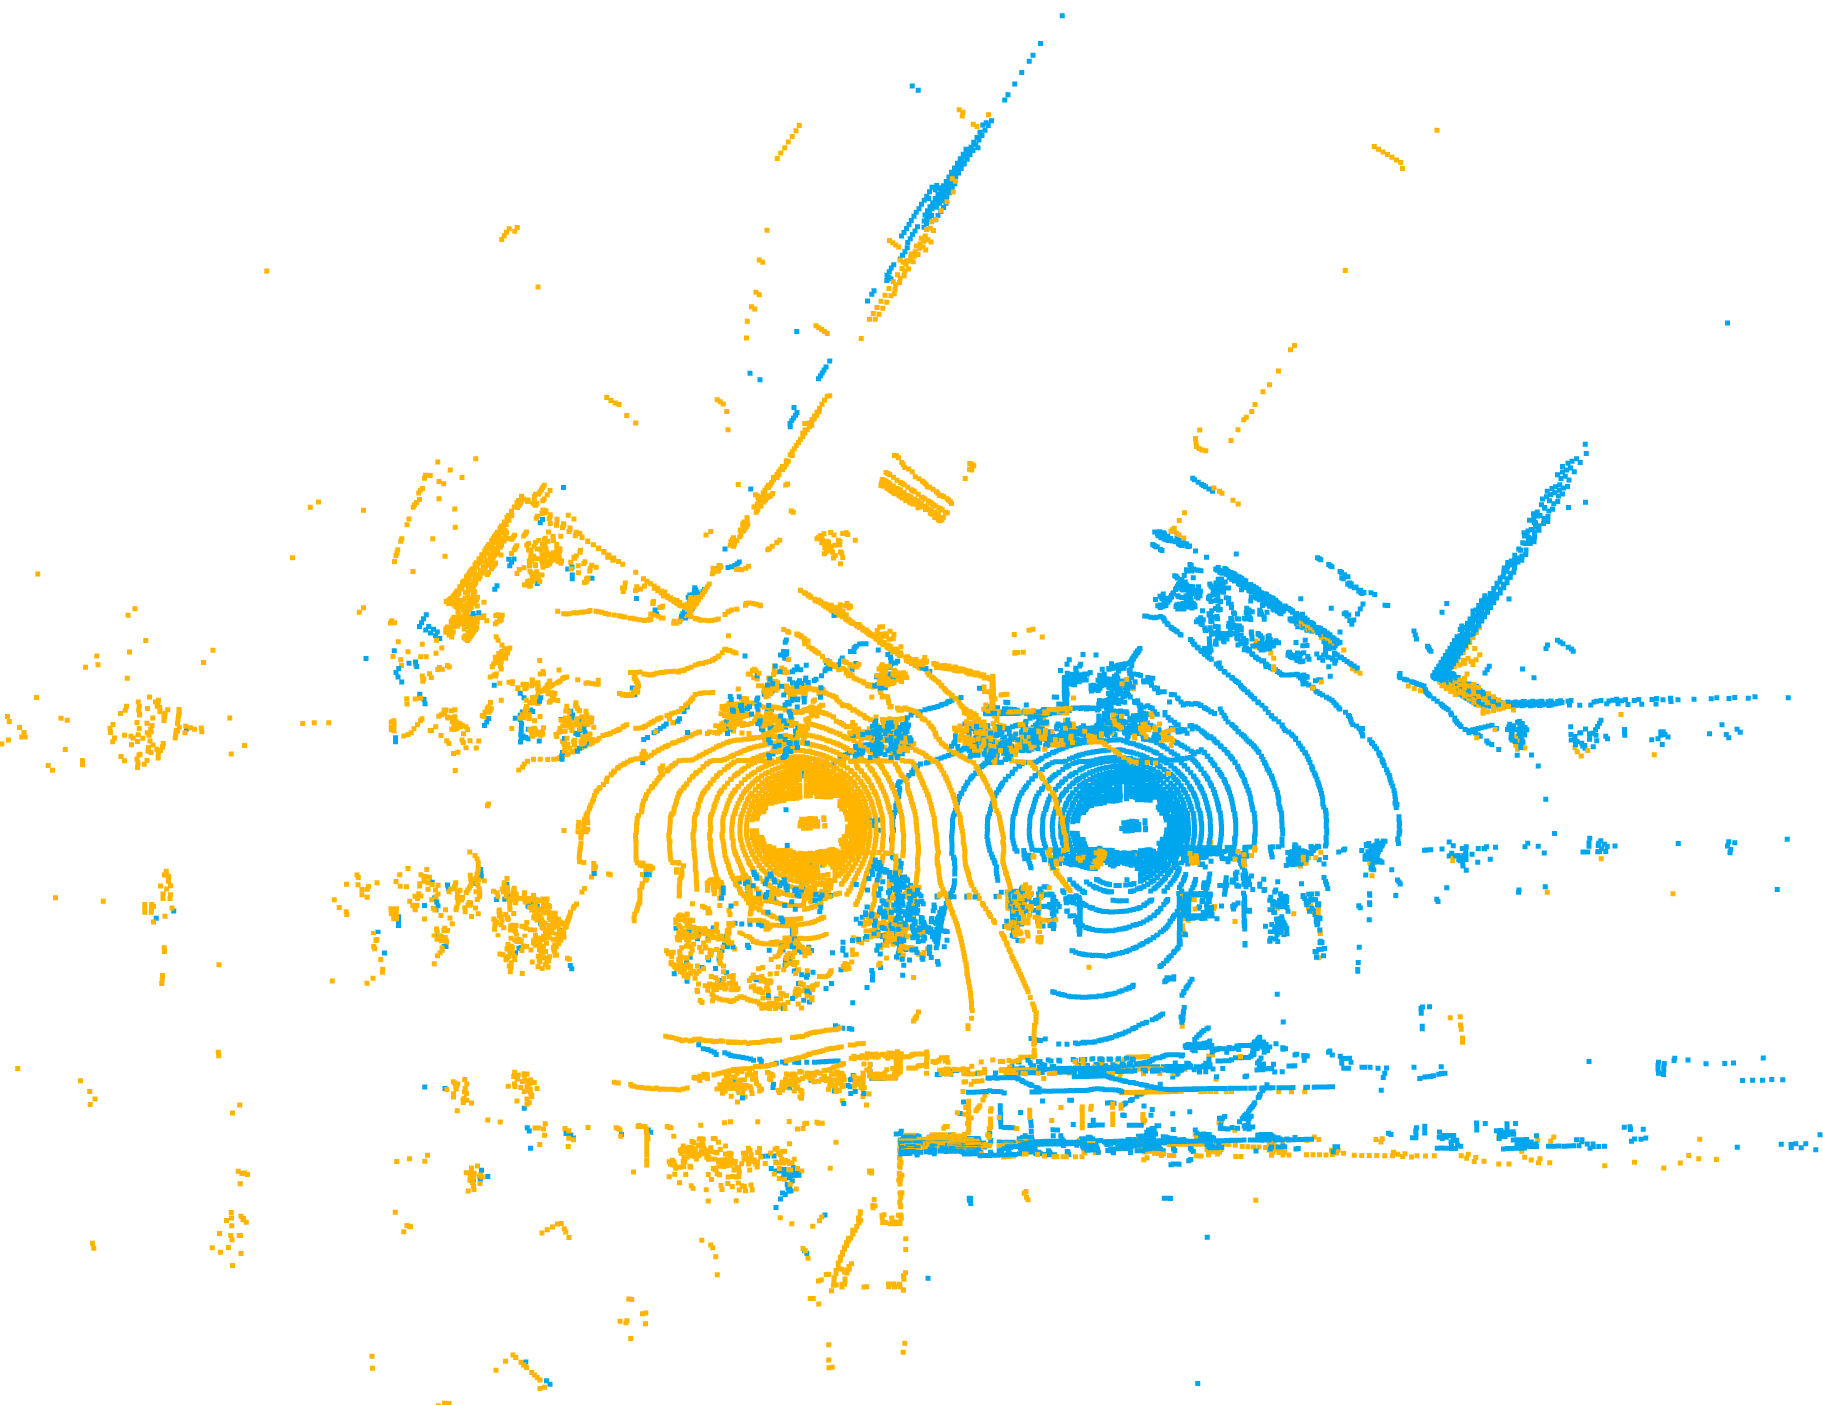} \hfill
  \includegraphics[width=0.45\linewidth]{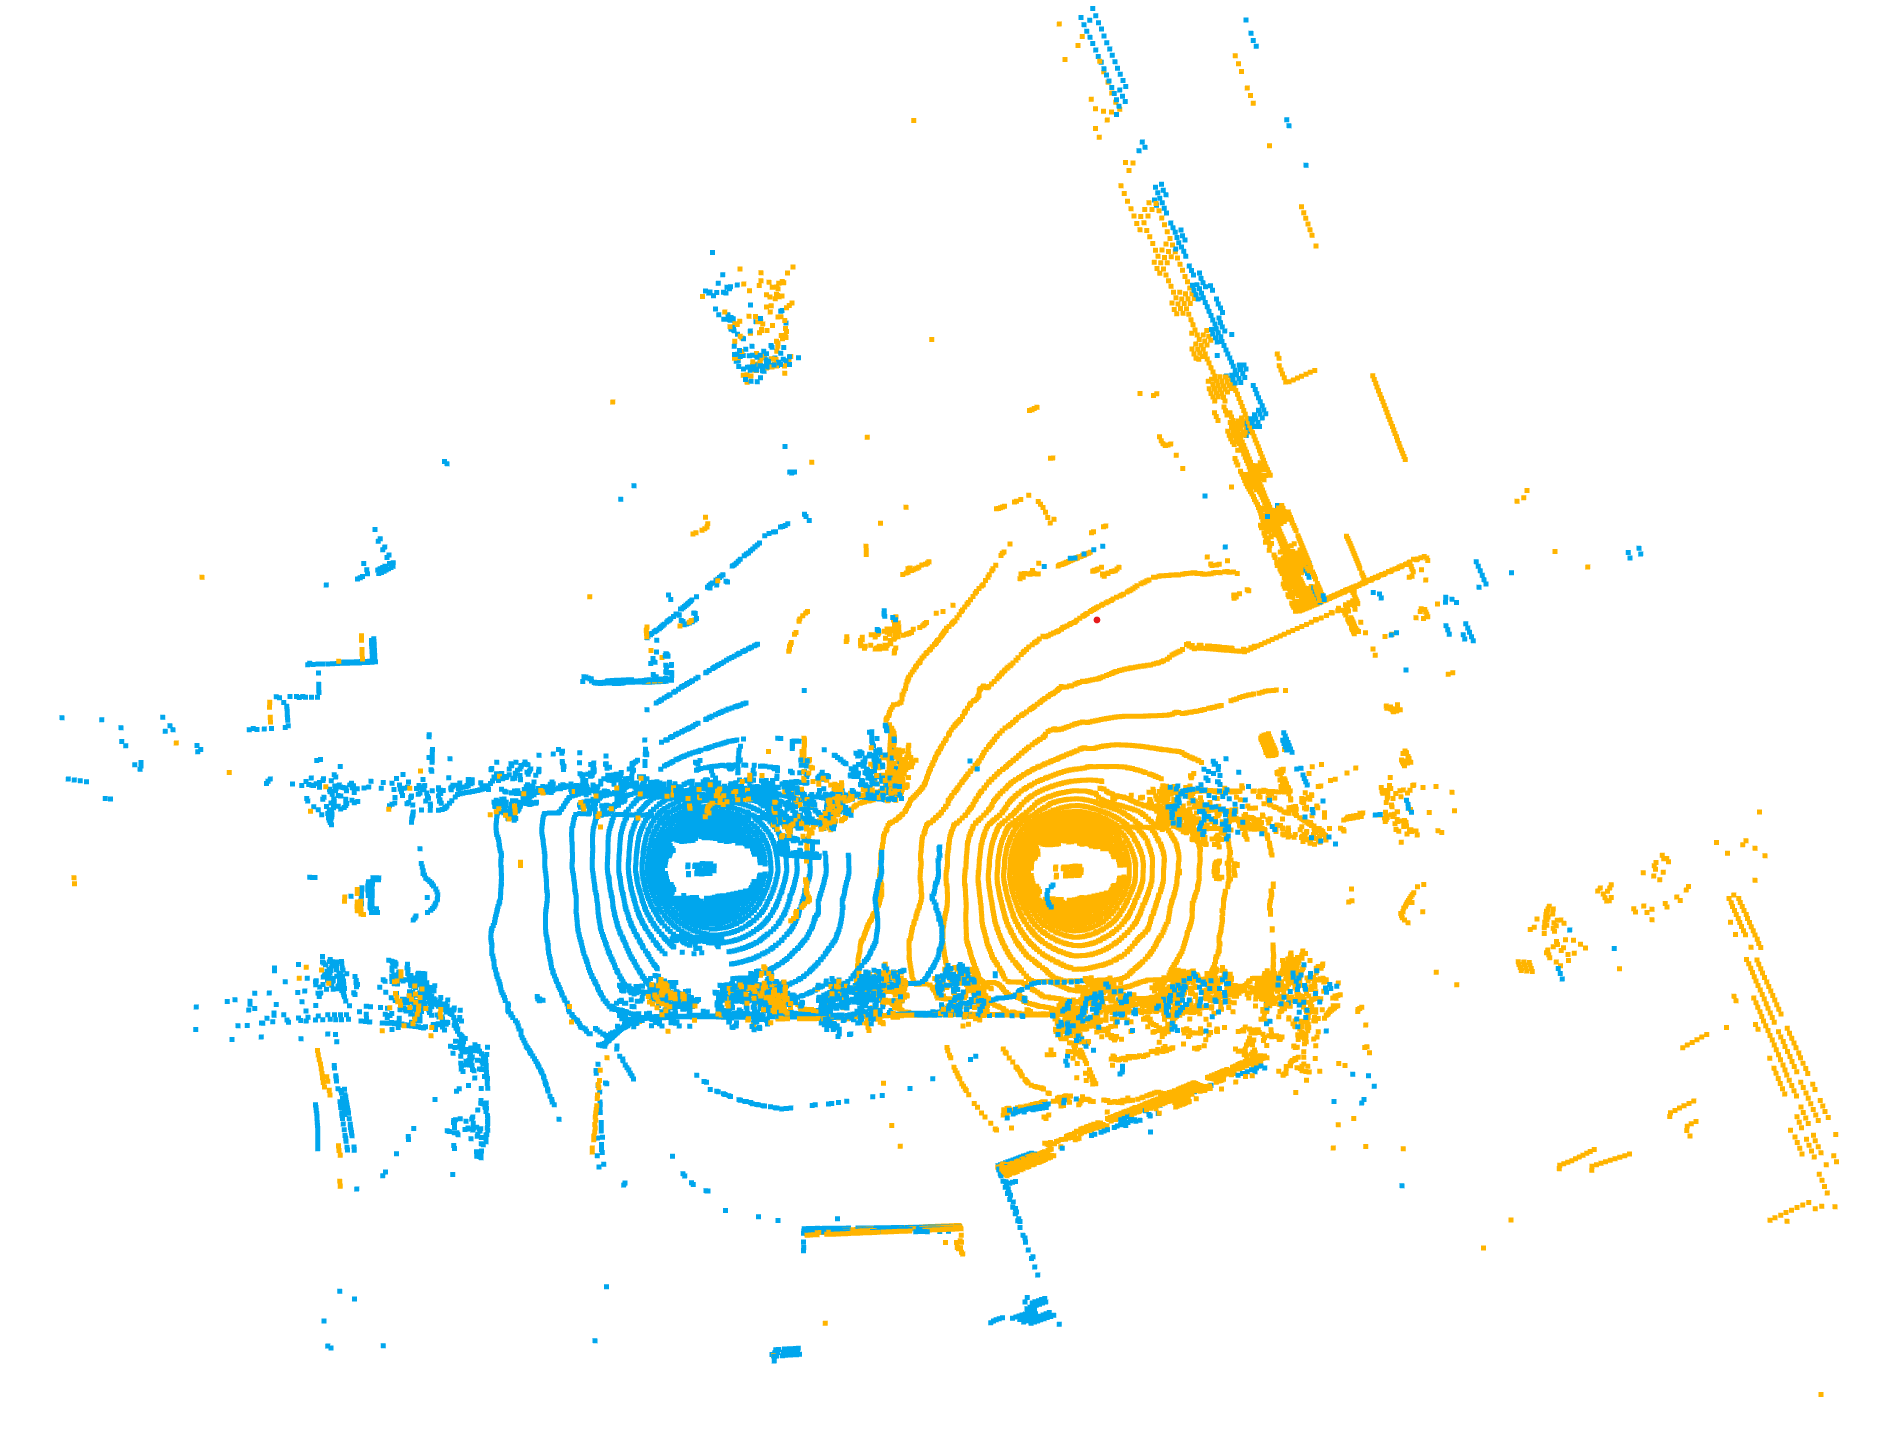} \hfill
  \caption{Registration results of EYOC on nuScenes \cite{Caesar_2020_CVPR}.}
  \label{fig:reg_results_nuscenes}
%   \vspace{-0.2cm}
\end{figure*}

\begin{figure*}[t]
  \centering
  \includegraphics[width=0.5\linewidth]{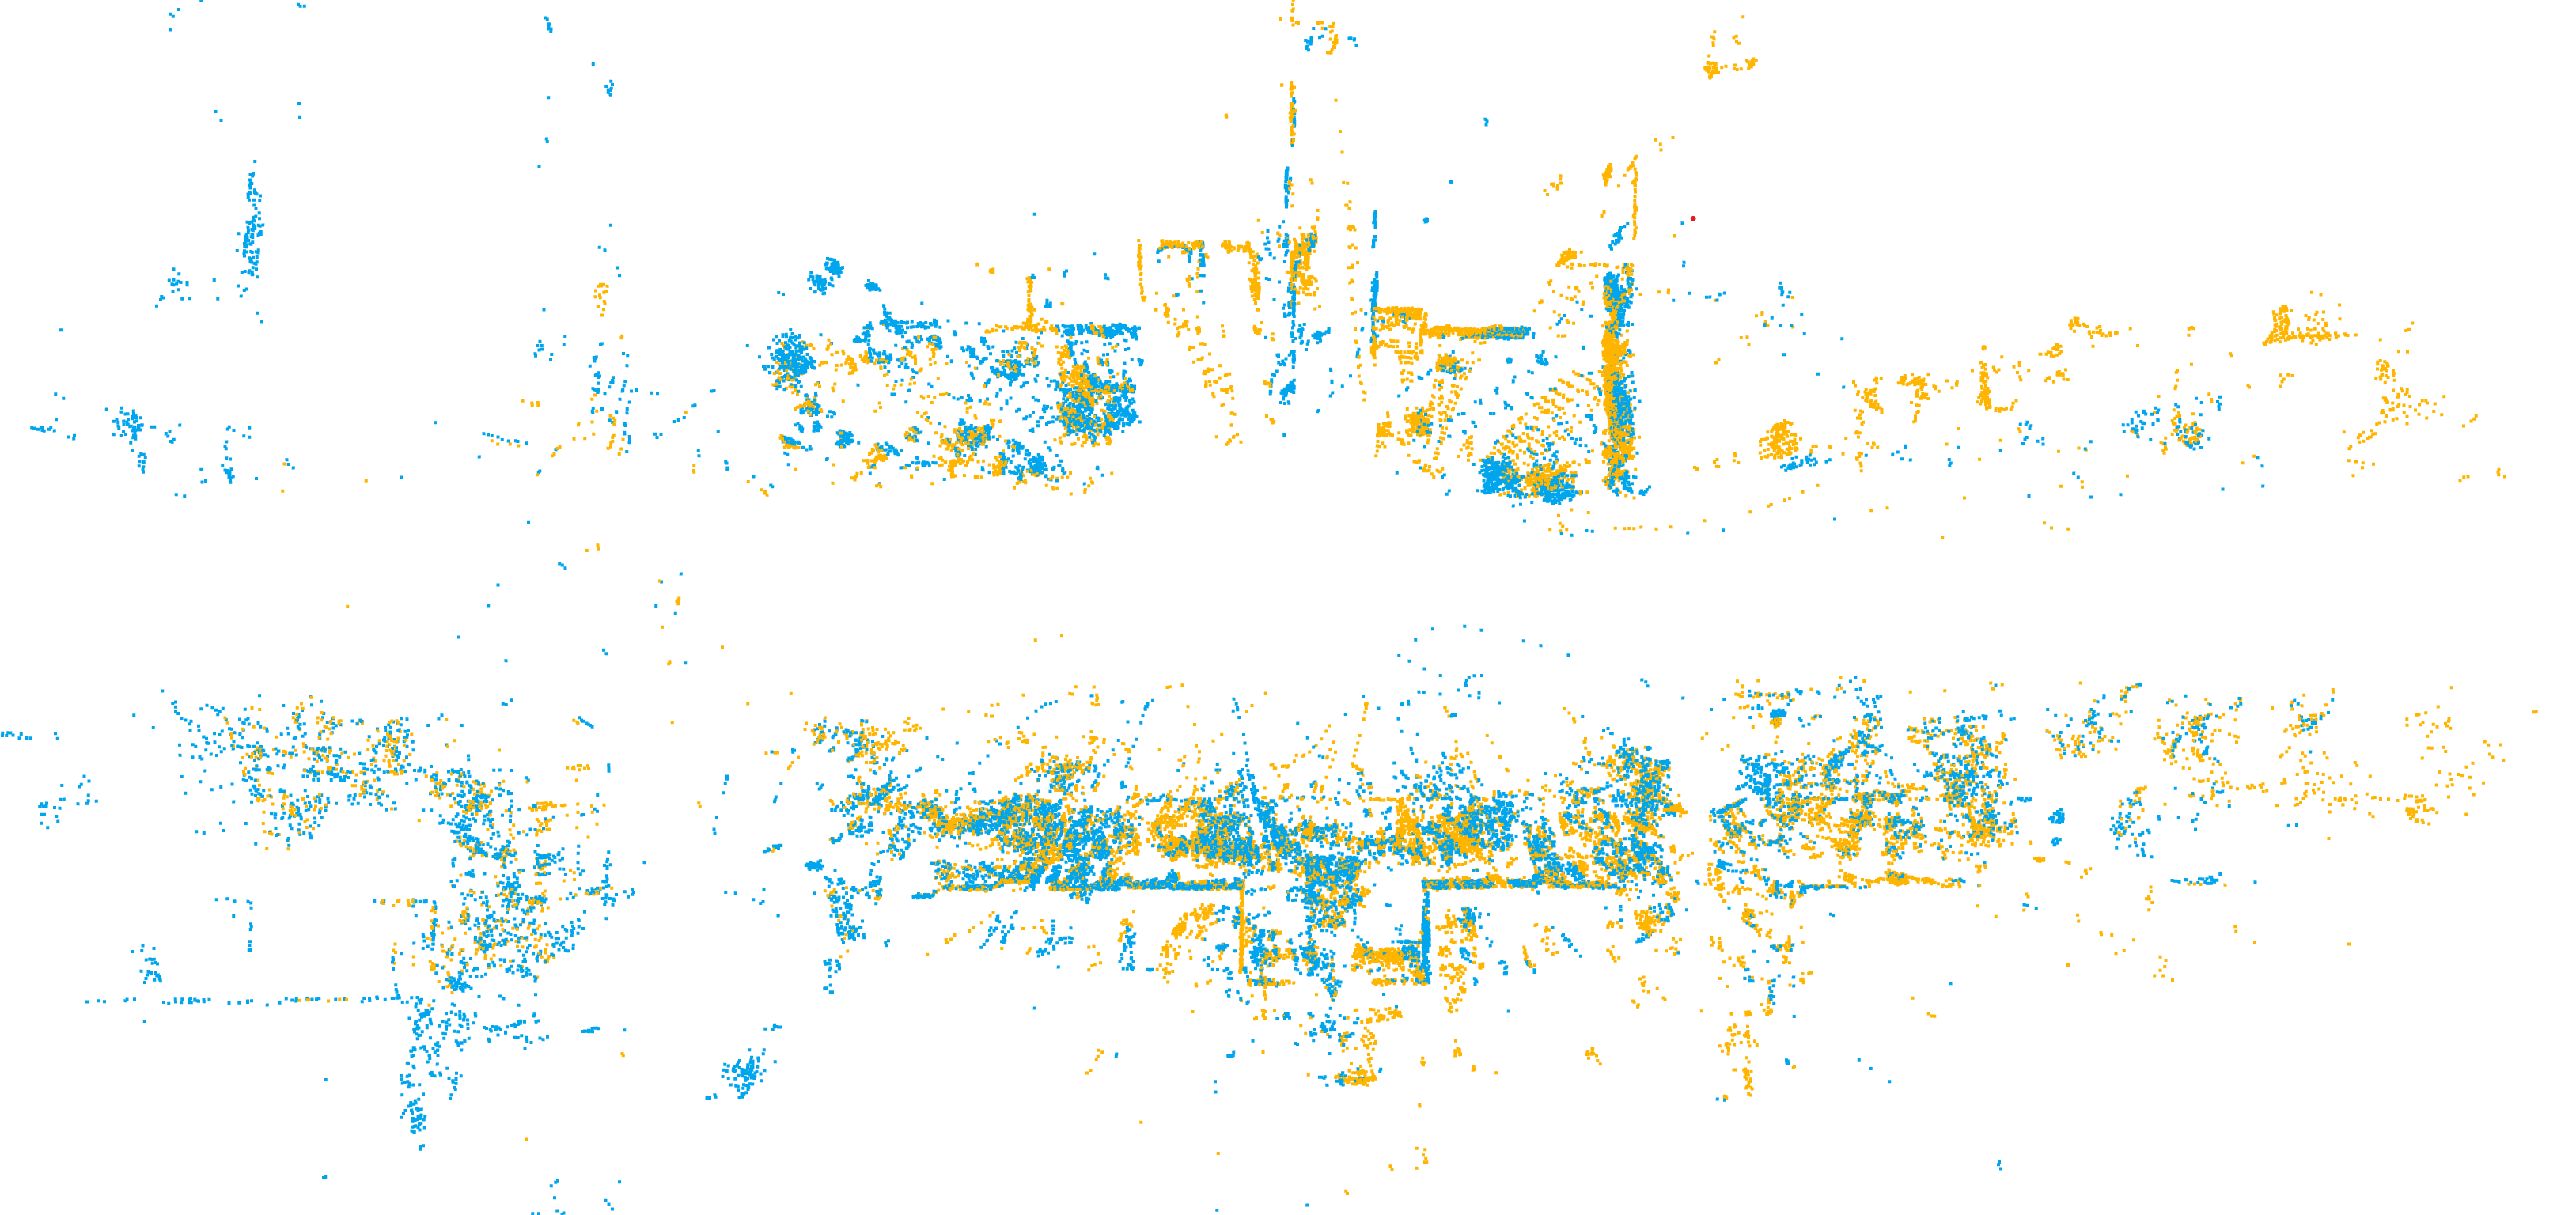} \hfill
  \includegraphics[width=0.45\linewidth]{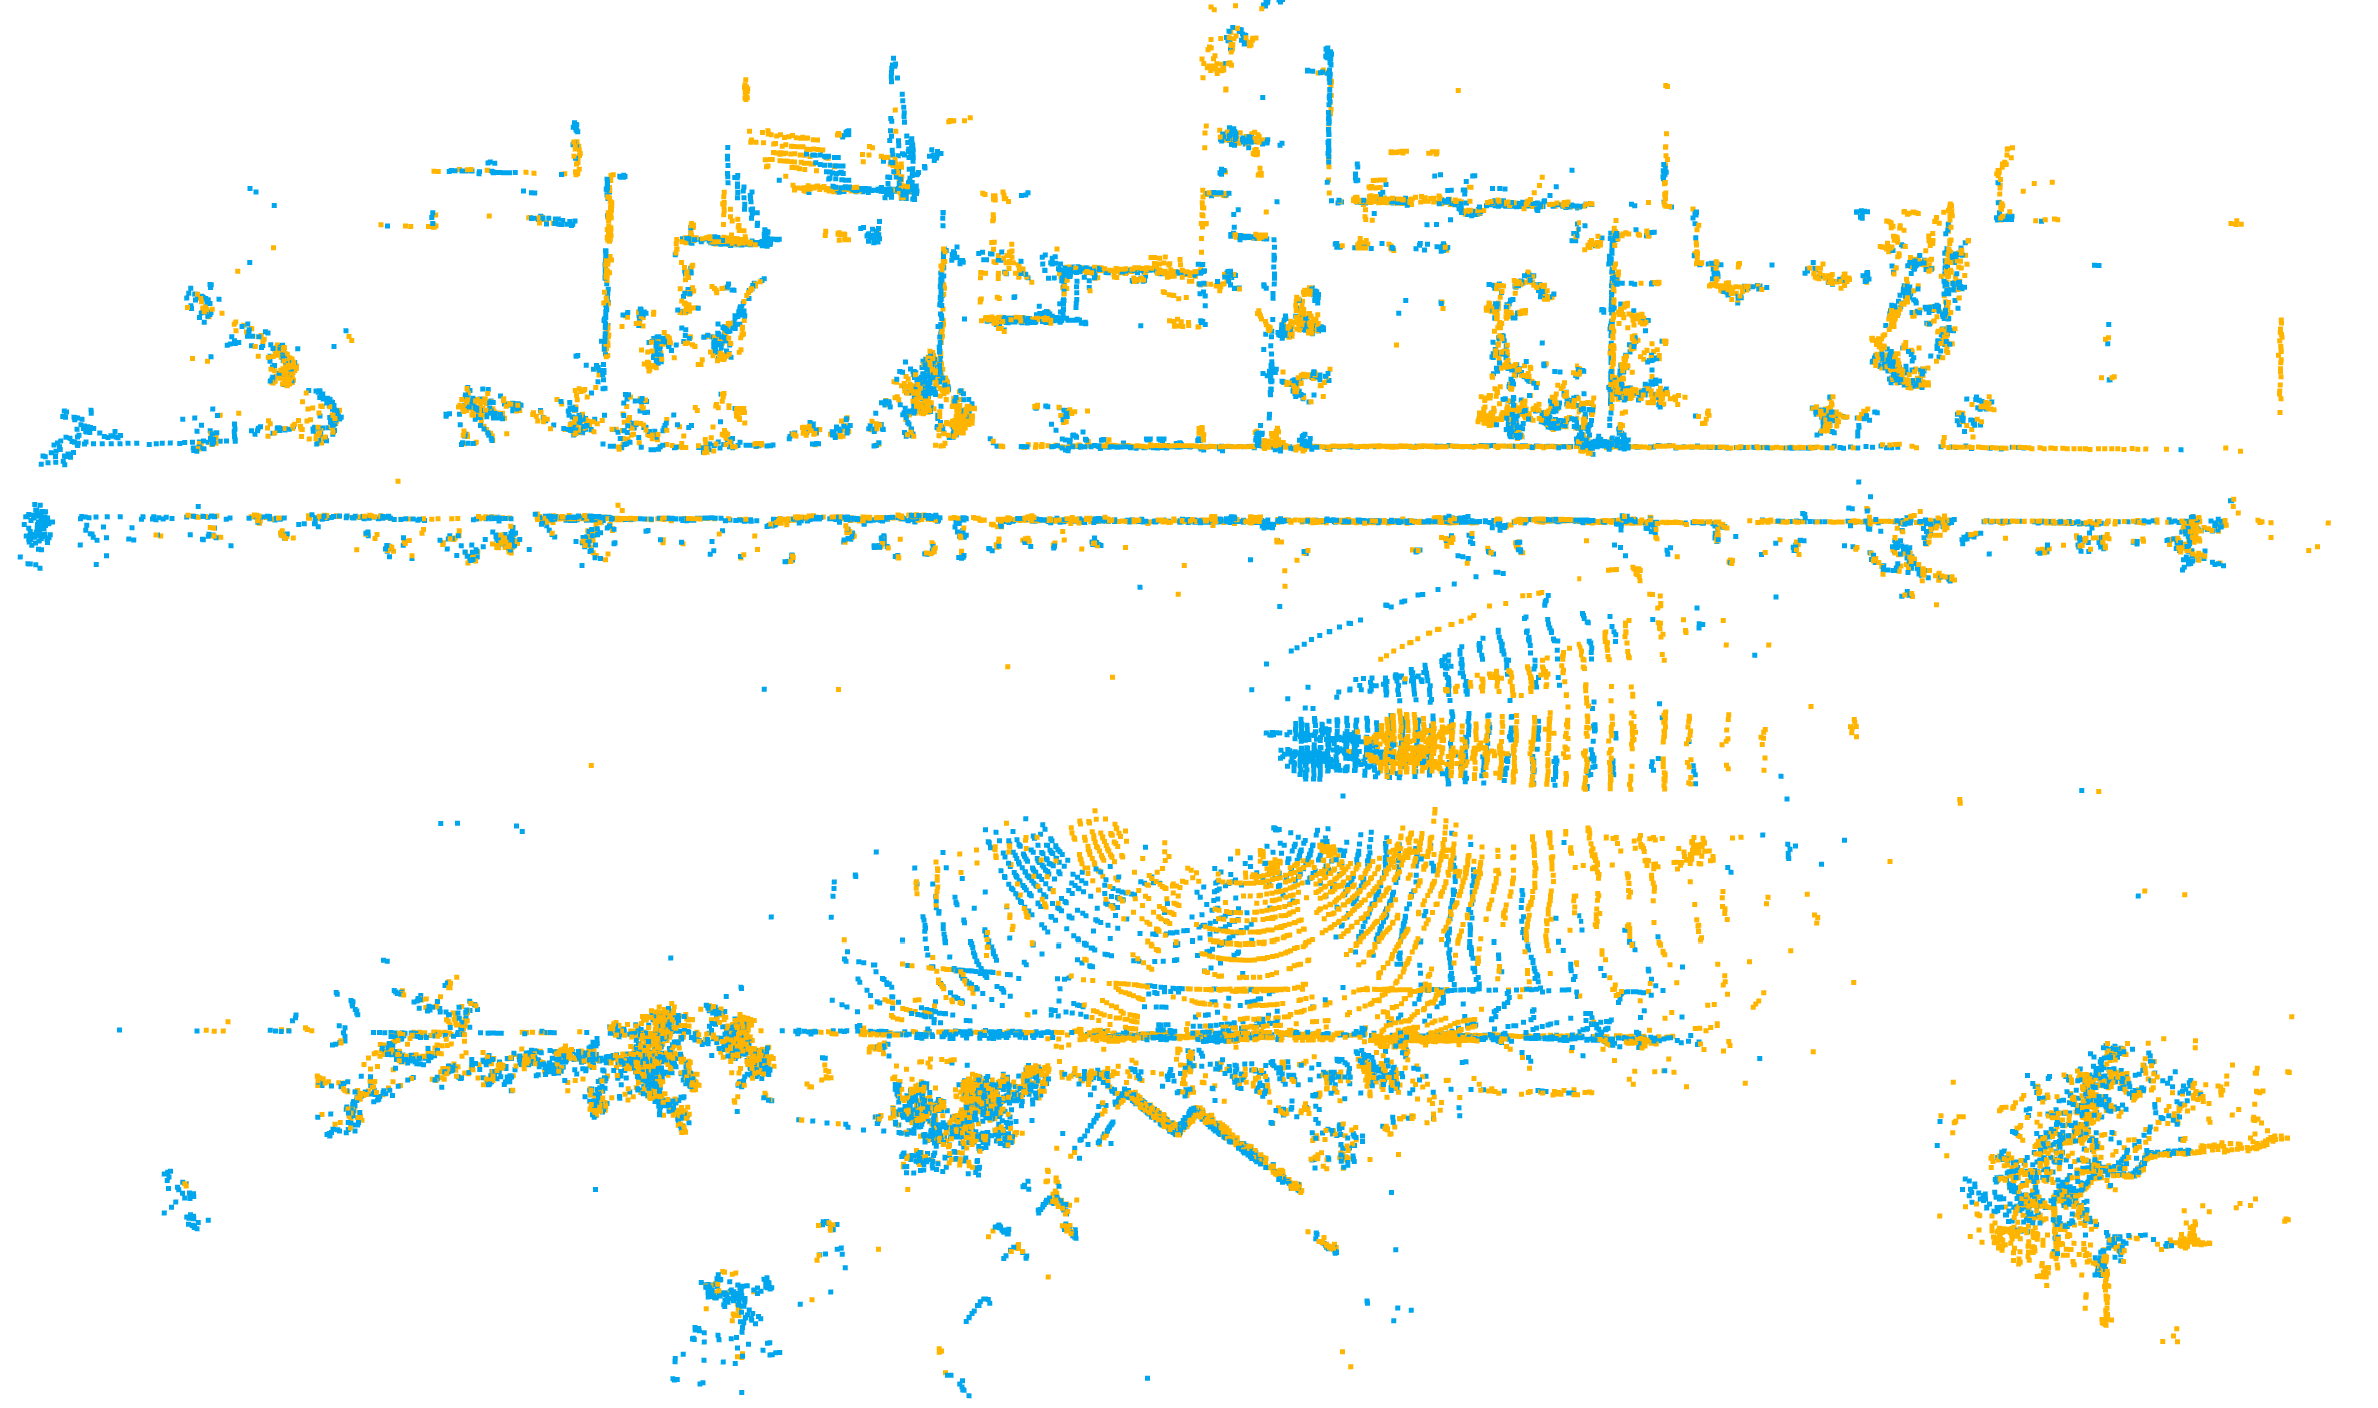} \hfill
  \caption{Registration results of EYOC on WOD \cite{Sun_2020_CVPR}.}
  \label{fig:reg_results_waymo}
%   \vspace{-0.2cm}
\end{figure*}
